# Supplementary material for: TextSR: Content-Aware Text Super-Resolution Guided by Recognition
Source: arXiv:1909.07113 source file (2019-10-20)
Supplement: Supplementary file 1 [file table_supple.tex]

\begin{center}
    \begin{tabular}{|c|ccccc|} 
    \hline
    \textbf{IC15}&&&&&\\
    \hline
    Size & 128$\times$32 & 64$\times$16 & 32$\times$8 & 24$\times$6 & 20\times5\\
    \hline
    BICUBIC & 74.8 & 73.8 & 38.2 & 16.2 & 7.2   \\
    SRGAN   & 74.9 & 74.8 & 52.0 & 28.3 & 15.0  \\
    TextSR  & \textbf{75.6} & 
    \textbf{75.1} & 
    \textbf{59.1} & 
    \textbf{37.7} & 
    \textbf{21.9} \\
    \hline
    Improve & +0.7 & +0.3 & +7.1 & +11.4 & +6.9\\
    \hline
    \hline
    \hline
    \textbf{IC03}&&&&&\\
    \hline
    Size & 128$\times$32 & 64$\times$16 & 32$\times$8 & 24$\times$6 & 20\times5\\
    \hline
    BICUBIC & 93.1 & 91.8 & 68.1 & 32.9 & 13.6   \\
    SRGAN   & 93.0 & 92.5 & 78.4 & 48.3 & 28.6  \\
    TextSR  & \textbf{93.2} & 
    \textbf{93.1} & 
    \textbf{85.0} & 
    \textbf{65.7} & 
    \textbf{43.7} \\
    \hline
    Improve & +0.2 & +0.6 & + 6.6 & +17.4 & +15.1\\
    \hline
    \textbf{IIIT5K}&&&&&\\
    \hline
    Size & 128$\times$32 & 64$\times$16 & 32$\times$8 & 24$\times$6 & 20\times5\\
    \hline
    BICUBIC & 92.4 & 89.9 & 58.3 & 28.0 & 13.7   \\
    SRGAN   & 92.1 & 91.6& 70.4 & 43.2 & 27.7  \\
    TextSR  & \textbf{92.5} & 
    \textbf{91.6} & 
    \textbf{77.9} & 
    \textbf{56.9} & 
    \textbf{40.9} \\
    \hline
    Improve & +0.4 & +0.0 & +7.5 & +13.7 & +13.2\\
    \hline
    \hline
    \textbf{CUTE}&&&&&\\
    \hline
    Size & 128$\times$32 & 64$\times$16 & 32$\times$8 & 24$\times$6 & 20\times5\\
    \hline
    BICUBIC & 78.8 & 71.9 & 33.3 & 12.5 & 6.2  \\
    SRGAN   & 77.4 & 74.4 & 47.6 & 23.3 & 10.4  \\
    TextSR  & \textbf{78.9} & 
    \textbf{75.3} & 
    \textbf{56.2} & 
    \textbf{34.7} & 
    \textbf{24.7} \\
    \hline
    Improve & +1.5 & +0.9 & +8.6 & +11.4 & +14.3 \\
    \hline
    \hline
    \textbf{SVT}&&&&&\\
    \hline
    Size & 128$\times$32 & 64$\times$16 & 32$\times$8 & 24$\times$6 & 20\times5\\
    \hline
    BICUBIC & 86.1 & 82.2 & 44.8 & 16.1 & 4.5   \\
    SRGAN   & 87.2 & 84.2 & 59.0 & 27.2 & 11.9  \\
    TextSR  & \textbf{87.2} & 
    \textbf{85.0} & 
    \textbf{67.5} & 
    \textbf{39.3} & 
    \textbf{22.3} \\
    \hline
    Improve & +0.0 & +0.8 & +8.5 & +12.1 & +10.2\\
    \hline
    \hline
    \textbf{SVTP}&&&&&\\
    \hline
    Size & 128$\times$32 & 64$\times$16 & 32$\times$8 & 24$\times$6 & 20\times5\\
    \hline
    BICUBIC & 76.7 & 71.2 & 31.6 & 11.6 & 2.8   \\
    SRGAN   & 77.1 & 74.0 & 46.2 & 23.7 & 11.0  \\
    TextSR  & \textbf{77.4} & 
    \textbf{75.8} & 
    \textbf{54.0} & 
    \textbf{31.0} & 
    \textbf{16.7} \\
    \hline
    Improve & +0.3 & +1.8 & +3.8 & +7.7 & +5.7\\
    \hline
    \end{tabular}
\end{center}
